# Supplementary material for: Focussing frustration for self-limiting assembly of flexible, curved particles
Source: arXiv:2203.03837 ancillary file (2022-03-08)
Supplement: Supplementary file 1 [file SI.pdf]

# Supporting information

## Contents

1 Continuum model of aligned, conformally-stacked curvamer energetics 1

2 Design of a curvamer 3

3 Measuring bending energy in simulation 5

4 Adhesion between two flat plates 6

5 Energy ratio, dimensionless parameters, and self-limiting size 7

6 Energy minimization methods 8

7 Radius of curvamers in a stack 9

8 Escape of curvamer stacking assembly 11

## 1 Continuum model of aligned, conformally-stacked curvamer energetics

Here, we describe the energetics of aligned, conformally-stacked curvamers. Specifically, we consider stacks of $N$ particles, each of which is assumed to obey the condition for perfect, conformal contact,

$$\kappa_{n+1} = \frac{\kappa_n}{1 + \kappa_n t}, \tag{S1}$$

where $\kappa_n$ is the curvature of the $n$th particle in the stack, and the $(n + 1)$th particle is attached to the convex face of the $n$th particle. Here we assume that curvature is *uniform* along the curvamer so that the condition of eq. (S1) implies that curvamers are concentrically stacked circular arcs throughout the stack, such that the curvature of all particles can be parameterized by the curvature

$\kappa_-$ of a fictitious $n = 0$ particle at the bottom of the stack,

$$\kappa_n = \frac{\kappa_-}{1 + \kappa_- n t}. \tag{S2}$$

From this the total elastic energy of the stack is simply,

$$E_{\rm el}(N, \kappa_-) = \frac{BA}{2} \sum_{n=1}^{N} \big(\kappa_n - \kappa_0\big)^2 \simeq \frac{BA}{2} \int_0^N dn \, \big(\kappa_n - \kappa_0\big)^2. \tag{S3}$$

where in the limit of $N \gg 1$ the discrete sum is well-approximated by the integral given on the right-hand side. To evaluate this, it is most convenient to define the reduced curvature $k \equiv \kappa_-/\kappa_0$ and the scaled height in the stack $h \equiv n\kappa_0 t$, such that the elastic energy takes the form,

$$E_{\rm el}(H, k) = \frac{BA\kappa_0}{2t} \int_0^H dh \, \Big(\frac{k}{1 + kh} - 1\Big)^2 = \frac{BA\kappa_0}{2t} \Big[\frac{H + kH(H + k)}{1 + kH} - 2\ln\big(1 + kH\big)\Big], \tag{S4}$$

where $H = N\kappa_0 t$ is the reduced stack size. For a given stack size the curvatures adjust to minimize the elastic energy, with an equilibrium determined by $\partial E_{\rm el}/\partial k = 0$, which has the solution $k_*(H)$,

$$k_*(H) = 1 - H^{-1} + \sqrt{H^{-2} + 1}. \tag{S5}$$

At the bottom of the stack the curvature varies from the preferred precurvature for short stacks (i.e. $k_*(H \to 0) \to 1$) to a maximal overcurvature at large stack sizes (i.e. $k_*(H \to \infty) \to 2$).

Inserting the size-dependent curvature into eq. (S4) yields the variation of elastic energy on stack size,

$$E_{\rm el}(H, k_*(H)) = \frac{BA\kappa_0}{2t} \Big[\frac{2\sqrt{H^2 + 1} - 2 + H^2}{H} - 2\sinh^{-1} H\Big]. \tag{S6}$$

Notably, this elastic energy exhibits superextensive growth for small stack sizes $E_{\rm el} \sim H^3$. This derives from the fact that for short stacks, bending strain varies linearly in the stack about a "neutral" central particle. For large stacks, constituent particles flatten with increased size, leading to an asymptotically constant elastic cost per particle $E_{\rm el} \sim H$.

Combining the size-dependent elastic energy with cohesive energy between the curvamers, we have the total stack energy,

$$E(N) = -\gamma A(N - 1) + E_{\rm el}(N), \tag{S7}$$

where $\gamma$ is the cohesive energy per unit length of curvature contact. To assess the size selectivity of

the competition between cohesion and elasticity, we consider the scaled energy per particle,

$$\frac{E(H)}{N} = BA\kappa_0^2\left(\frac{S}{H} + \frac{1}{2}\left[\frac{2\sqrt{H^2+1} - 2 + H^2}{H^2} - \frac{2}{H}\sinh^{-1} H\right]\right) - \gamma w, \tag{S8}$$

where

$$S \equiv \frac{\gamma t}{B\kappa_0} \tag{S9}$$

is the reduced cohesion. For a given $S$ the equilibrium stack size is determined by the minimum of eq. (S8) with respect to $H$, yielding an equation of state relating optimal stack size $H_*$ to cohesion,

$$S(H_*) = \frac{2 - 2\sqrt{H_*^2+1}}{H_*} + \sinh^{-1} H_* \tag{S10}$$

This relationship exhibits a power law relationship at small size, $S \sim H_*^3$, corresponding to $H_* \sim S^{1/3}$. Whereas in the large stack limit, $S \sim \ln 2H_*$, corresponding to an exponential growth of stack size with cohesion $H_* \sim e^S$

## 2 Design of a curvamer

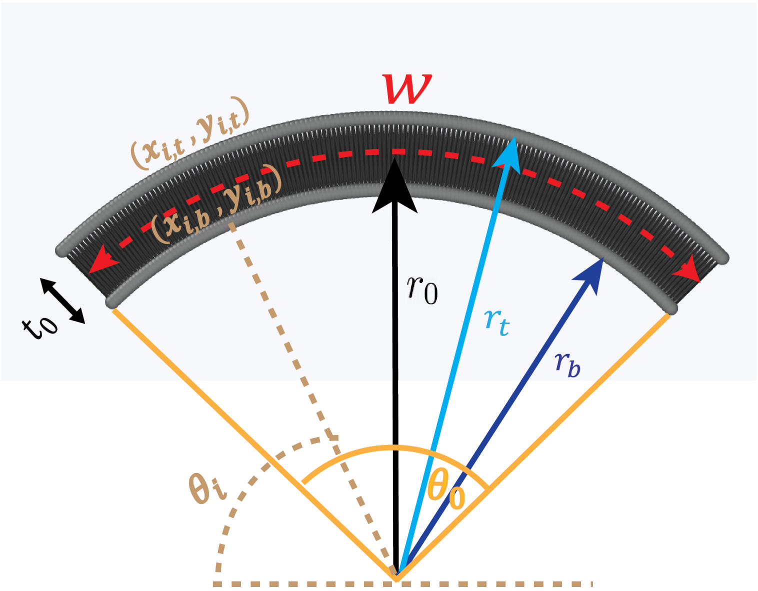


Figure S1: Structure of a curvamer.

The geometry of a curvamer is determined from three independent parameters, $r_0$, $\theta_0$, and $t_0$ as shown in table S1. Design 1, design 2, and design 3 represent the curvamers on Fig. 3c of the main manuscript.

Table S1: Radius, thickness, and width of curvamers

| Parameter | Design 1 | Design 2 | Design 3 |
|---|---|---|---|
| $r_0$ | 30 | 60 | 90 |
| $\theta_0$ (°) | 90 | 45 | 30 |
| $t_0$ | 5.0 | 5.0 | 5.0 |
| $w = r_0\theta_0$ | 47.124 | 47.124 | 47.124 |

To calculate the Cartesian coordinates of the beads in the curvamer, their corresponding polar angles $\theta_i$ were calculated from the total angular envelope $\theta_0$. From the minimum angle $\theta_{\min} = 90 - \frac{\theta_0}{2}$ and the maximum angle $\theta_{\max} = 90 + \frac{\theta_0}{2}$, we find $\theta_i = \theta_{\min} + i\frac{\theta_{\max} - \theta_{\min}}{n-1}$, where $n = 150$. The radius of curvature of the first bead layer, $r_b = r_0 - \frac{t_0}{2}$ and the radius of curvature of the second bead layer, $r_t = r_0 + \frac{t_0}{2}$. From these values, the positions of all beads on both of the layers are calculated as described below.

Beads on the first layer:

$$x_{i,b} = A + r_b cos(\theta_i), \tag{S11}$$

$$y_{i,b} = B - \frac{t_0}{2} - r_b(1 - sin(\theta_i)) \tag{S12}$$

Beads on the second layer:

$$x_{i,t} = A + r_t cos(\theta_i) \tag{S13}$$

$$y_{i,t} = B + \frac{t_0}{2} - r_t(1 - sin(\theta_i)), \tag{S14}$$

where $(A, B)$ is the center of the curvamer.

The spring constants are chosen to match the elastic response of a thin isotropic plate of thickness $t_0$, Young's modulus $E$ and Poisson's ratio $\nu$, derived for the flat case $\kappa_0 = 0$. The moduli of such a plate associated with uniform bending, stretching and shear deformations are $B = Et_0^3/(12(1 - \nu^2)), Y = Et_0/(1 - \nu^2)$ and $S = Et_0/(2(1 + \nu))$, respectively. The deformations are related to the spring deformations of each trapepezoidal unit cell within the particle: bending strain $\kappa$ results in elastic energy per unit cell

$$E_{bend} = \frac{1}{4} d^2 h^2 k_h \kappa^2, \tag{S15}$$

for transverse stretching ratio $\epsilon$

$$E_{stretch} = \frac{d^4(k_c + k_h) + d^2h^2k_h(2k_c + k_v)}{d^2k_v + h^2(2k_c + k_v)}\epsilon^2 \tag{S16}$$

Table S2: Bead spacing, Poisson's ratio, and spring constant ratio

| Parameter | Value |
|---|---|
| $d$ | 0.3163 |
| $\nu$ | 0.3 |
| $\frac{k_v}{k_h}$ | 2.1044 |
| $\frac{k_c}{k_h}$ | 1.0542 |

and shear $\sigma$,

$$E_{shear} = \frac{d^2h^2}{d^2+h^2}k_c\sigma^2. \tag{S17}$$

From these three relations, conditions on the ratio of spring constants are

$$\frac{k_v}{k_h} = \frac{12t_0^2(1-\nu)}{4t_0^2 - 3d^2(1-\nu)} \tag{S18}$$

and

$$\frac{k_c}{k_h} = \frac{3(t_0^2+d^2)(1-\nu)}{2t_0^2}, \tag{S19}$$

where $d$ is the average distance between the beads and $\nu$ is the Poisson's ratio of the curvamer. Since the distance between the beads of the top ($d_t$) layer and the bottom layer ($d_b$) are different in the isosceles trapezoid, when $\kappa_0 > 0$ as shown in Fig. 2a, we consider the mean distance, $d_{\text{avg}} = d = \frac{d_b+d_t}{2}$, calculated from the bead positions. We keep the ratios $\frac{k_v}{k_h}$ and $\frac{k_c}{k_h}$ constant for all curvamer designs and bending moduli.

# 3 Measuring bending energy in simulation

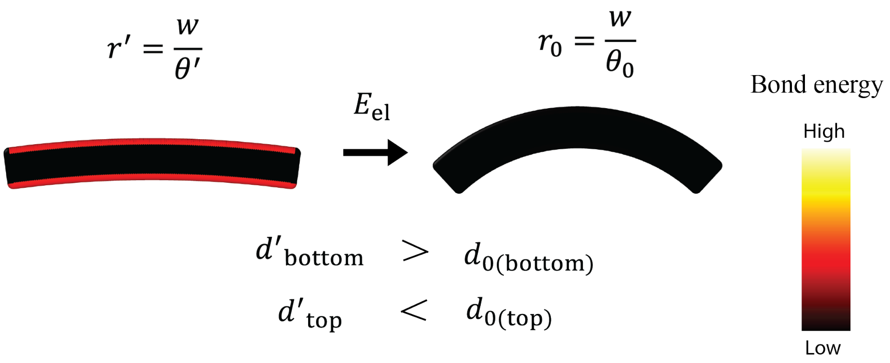


Figure S2: Bond energy mapping of a flattened curvamer that relaxes to its ground state. The higher bond energy at the initial state is shown by the red color. The bottom layer of the beads is stretched and the top layer of the beads is compressed in this state.

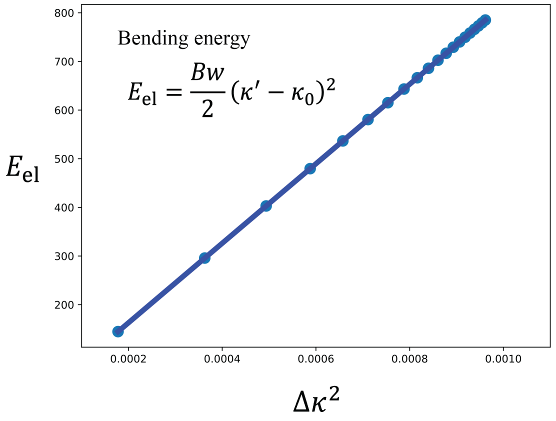


Figure S3: Linear elastic bending of a model curvamer demonstrated by the bending energy plot achieved from bending simulations.

To prepare a curvamer with a radius of curvature $r'$ that is different from its preferred radius $r_0$, we calculate its new angular envelope $\theta' = \frac{w}{r'}$. Then we find the coordinates of the beads following the equations S11-S14. When the curvamer relaxes from a flat state to a curved state with preferred $r_0$, the first (bottom) layer of the beads shrinks and the second (top) layer of the beads expands. We measure the bending energy in the simulation by relaxing a curvamer from different flattened states (different $r'$ values) and confirm its linear relationship with increasing $(\Delta\kappa)^2$, (where $\Delta\kappa = \frac{1}{r_0} - \frac{1}{r'}$), that resembles a linear elastic material.

# 4 Adhesion between two flat plates

The total interaction potential between two flat plates are calculated by taking the sum of all the inter-bead potentials.

$$\gamma A = \sum_{i=1}^{n} \sum_{j=1}^{n} 4\epsilon \left[ \left( \frac{\sigma}{r_{\text{ij}} - \Delta} \right)^{12} - \left( \frac{\sigma}{r_{\text{ij}} - \Delta} \right)^{6} \right] \tag{S20}$$

The yellow-magenta pairs contribute to the total plate potential significantly as their interaction strength $\epsilon$ is much larger than the interaction strength between red-blue pairs $\epsilon' < 0.0001\epsilon$ where $\epsilon'$ is the repulsive interaction coefficient.

**Choice of potential parameters** To keep the equilibrium separation distance ($t = t_0 + r_* = 1.71t_0$) and the total adhesion energy ($\gamma A$) between the plates constant for all different potential ranges $\sigma$, as shown in Fig. 2c in the main text, we adjusted the $\Delta$ and the $\epsilon$ parameters of the inter-bead potentials to maintain constant $t$ and $\gamma A$.

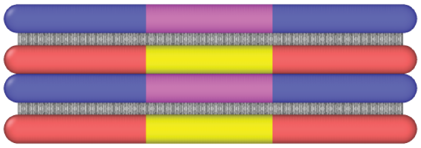


Figure S4: Adhesion energy $\gamma A$ is calculated by integrating the LJ-potential between the beads at top layer of plate 1 and the bottom layer of plate 2.

The values of the inter-bead LJ-potental parameters used in the simulations are listed below.

Table S3: Short-ranged interaction $\sigma_1 = 0.06t$

| Potential type | Parameter | Value |
|---|---|---|
| Attractive | $\sigma_1$ | 0.5 |
| | $\Delta_1$ | 3.02 |
| | $\epsilon_1$ | 3.0 |
| Repulsive | $\sigma_1'$ | 0.5 |
| | $\Delta_1'$ | 3.2 |
| | $\epsilon_1'$ | 0.0001 |

Table S4: Medium-ranged interaction $\sigma_2 = 0.12t$

| Potential type | Parameter | Value |
|---|---|---|
| Attractive | $\sigma_2$ | 1.0 |
| | $\Delta_2$ | 2.5 |
| | $\epsilon_2$ | 2.1 |
| Repulsive | $\sigma_2'$ | 1.0 |
| | $\Delta_2'$ | 2.7 |
| | $\epsilon_2'$ | 0.0001 |

## 5 Energy ratio, dimensionless parameters, and self-limiting size

The values of the spring constants, bending energy, adhesion energy, dimensionless parameters, and self-limiting stack size shown in plots of Fig. 3c and Fig. 4a of the main text are listed in tables S6 and S7.

Table S5: Long-ranged interaction $\sigma_3 = 0.18t$

| Potential type | Parameter | Value |
|---|---|---|
| Attractive | $\sigma_3$ | 1.5 |
| | $\Delta_3$ | 2.0 |
| | $\epsilon_3$ | 1.7 |
| Repulsive | $\sigma_3'$ | 1.5 |
| | $\Delta_3'$ | 2.1 |
| | $\epsilon_3'$ | 0.0001 |

Table S6: Simulation parameters used in Fig. 3c

| Parameter | Design 1 | Design 2 | Design 3 |
|---|---|---|---|
| $r_0$ | 30(3.5t) | 60(7.0t) | 90(10.5t) |
| $\sigma$ | 0.06t | 0.06t | 0.06t |
| $k_h$ | $2.00 \times 10^3 - 3.98 \times 10^4$ | $6.31 \times 10^3 - 1.0 \times 10^5$ | $2.00 \times 10^4 - 3.16 \times 10^5$ |
| $BA$ | $7.42 \times 10^5 - 1.48 \times 10^7$ | $2.34 \times 10^6 - 3.73 \times 10^7$ | $7.42 \times 10^6 - 1.18 \times 10^8$ |
| $\gamma A$ | $1.00 \times 10^3$ | $9.97 \times 10^2$ | $3.31 \times 10^2$ |
| $\frac{\gamma}{B}$ | $1.00 \times 10^{-3} - 6.8 \times 10^{-5}$ | $4.00 \times 10^{-4} - 2.68 \times 10^{-5}$ | $4.46 \times 10^{-5} - 2.81 \times 10^{-6}$ |
| $S$ | $0.34 - 0.02$ | $0.22 - 0.01$ | $0.03 - 0.002$ |
| $N_{\text{min}}$ | $14 - 3$ | $19 - 5$ | $10 - 5$ |
| $H$ | $3.96 - 0.85$ | $2.69 - 0.71$ | $0.94 - 0.47$ |

Table S7: Simulation parameters used in Fig. 4b

| Parameter | Range 1 | Range 2 | Range 3 |
|---|---|---|---|
| $r_0$ | 30(3.5t) | 30(3.5t) | 30(3.5t) |
| $\sigma$ | 0.06t | 0.12t | 0.18t |
| $k_h$ | $8.81 \times 10^2 - 3.98 \times 10^4$ | $2.15 \times 10^3 - 3.98 \times 10^4$ | $5.29 \times 10^3 - 3.98 \times 10^4$ |
| $BA$ | $3.27 \times 10^5 - 1.48 \times 10^7$ | $7.98 \times 10^5 - 1.48 \times 10^7$ | $1.97 \times 10^6 - 1.48 \times 10^7$ |
| $\gamma A$ | $1.00 \times 10^3$ | $1.00 \times 10^3$ | $1.00 \times 10^3$ |
| $\frac{\gamma}{B}$ | $3.00 \times 10^{-3} - 6.83 \times 10^{-5}$ | $1.3 \times 10^{-3} - 6.83 \times 10^{-5}$ | $5.1 \times 10^{-4} - 6.83 \times 10^{-5}$ |
| $S$ | $0.78 - 0.02$ | $0.32 - 0.02$ | $0.14 - 0.02$ |
| $N_{\text{min}}$ | $69 - 3$ | $39 - 3$ | $25 - 4$ |
| $H$ | $19.55 - 0.85$ | $11.05 - 0.85$ | $7.08 - 1.13$ |

# 6 Energy minimization methods

The initial state of a curvamer stack is prepared so that the first curvamer at the bottom of the stack is in its preferred radius $r_0$ and the subsequent curvamers have increasing radii of curvature $r_n = r_{n-1} + t$, as shown in Fig. S5.

**Conjugate gradient algorithm** Energy minimization was implemented by using the built-in Polak-Ribiere version of the conjugate gradient (CG) algorithm in LAMMPS (`https://docs.lammps.org/minimize.html`). The stopping tolerance for energy, stopping tolerance for force, maximum iterations of minimizer, and maximum number of force/energy evaluations were set to $10^{-12}$, $10^{-12}$, $10^5$, and $5 \times 10^4$.

**Simulated Annealing** We utilize langevin dynamics to control the system's temperature over the course of the simulation `https://docs.lammps.org/fix_langevin.html`. The curvamers were cooled from $T_i = 1.2\epsilon/k_B$ to $T_f = 0.0001\epsilon/k_B$ over a period of $10^6$ iterations, where each iteration represents a time step of $\tau = 0.001s$. During each time step, the mean squared displacement of each particle is $d^2 = 4D\tau = 4\frac{k_BT}{\gamma_{drag}}\tau = 0.5 \times 10^{-4}t^2(k_BT)$.

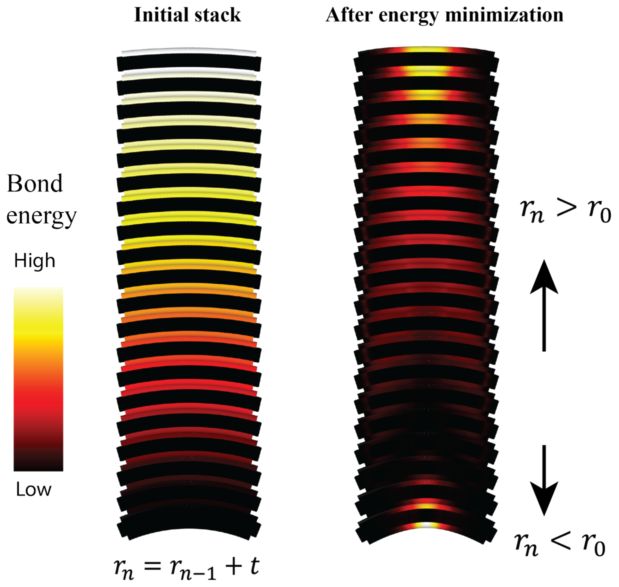


Figure S5: The initial (left) and the minimum-energy final (right) state of a curvamer stack.

## 7 Radius of curvamers in a stack

We measure the radius of curvature of each curvamer in a stack $r_n$ from the positions of the bead pairs. First, we find the midpoints of the line segments that connect the beads of the top layer $(P_1, Q_1, R_1, ...)$ to the beads of the bottom layer $(P_2, Q_2, R_2, ...)$. From the coordinates of every three midpoints (as shown by $P, Q, R$ on the left panel of Fig. S7), we calculate a local radius of curvature. Finally, we calculate the average of all local radii measured from the points $(1, 2, 3), (2, 3, 4), (3, 4, 5), ..., (48, 49, 50)$ (as shown in the right panel of Fig. S7) that represents the

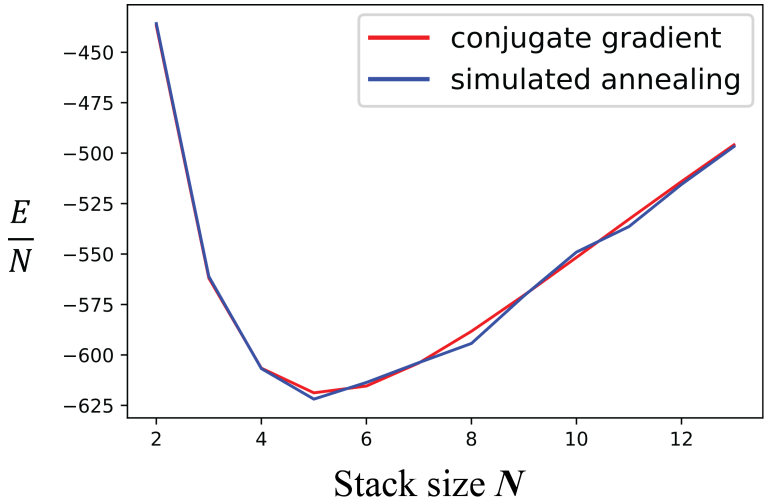


Figure S6: Energy density plot calculated using conjugate gradient algorithm and simulated annealing method show good agreement, both resulted in the energy minimum at $N = 5$.

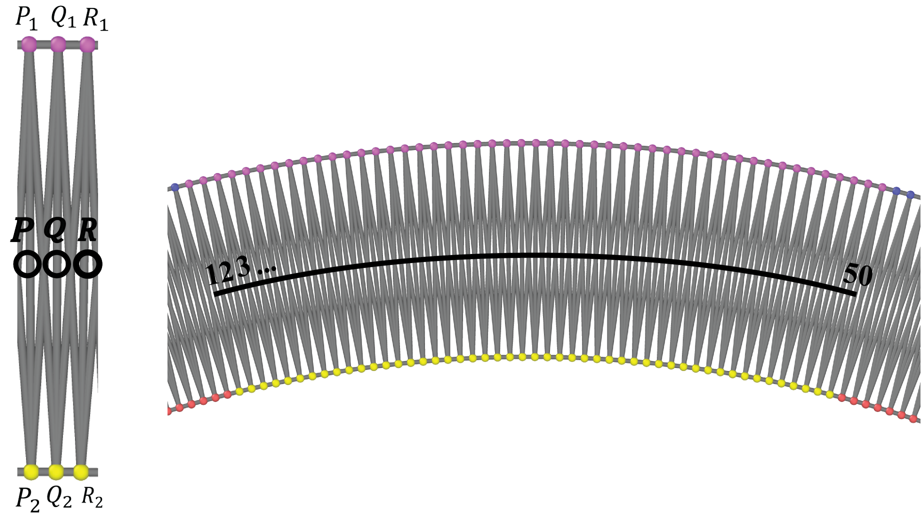


Figure S7: Left panel: the midpoints (P,Q,R) of the line segments connecting the beads on the two layers of a model curvamer. Right panel: All the midpoints in the patchy region of the curvamer, from which the average radius of curvature $r_n$ is calculated.

mean radius of curvature of the curvamer, $r_n$.

The local radius $r_i$, the inverse of the Menger curvature, is calculated from the equation

$$r_i = \frac{\sqrt{[(x_1 - x_2)^2 + (y_1 - y_2)^2].[(x_2 - x_3)^2 + (y_2 - y_3)^2].[(x_3 - x_1)^2 + (y_3 - y_1)^2]}}{2.|(x_2 - x_1).(y_3 - y_2) - (y_2 - y_1).(x_3 - x_2)|}, \qquad \text{(S21)}$$

where $P(x_1, y_1), Q(x_2, y_2), R(x_3, y_3)$ are the coordinates of the three midpoints.

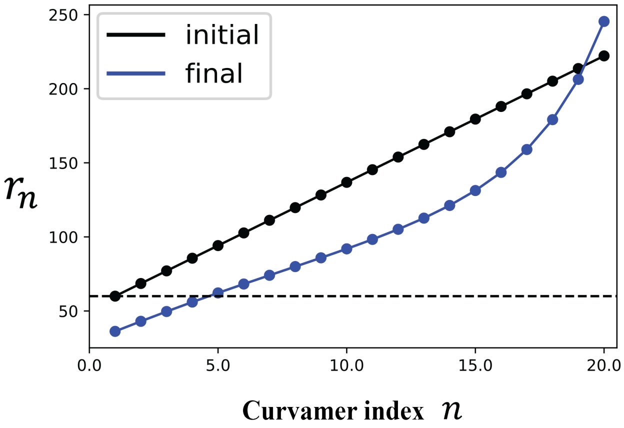


Figure S8: The radii of curvature of each curvamer in a stack of $N = 20$ as a function of their position index. The black plot shows the curvature at the initial state and the blue plot shows the curvature calculated at the ground state after energy minimization. The horizontal dashed line shows the preferred radius of curvature, $r_0 = 60$.

# 8 Escape of curvamer stacking assembly

The gap between the curvamers in two representative curvamer stack assemblies (shown in Fig. 4b of the main manuscript) is measured. We define this gap as $\delta'$ and show that the ratio of this gap to the maximum gap $\delta$ increases in the case of long-ranged interaction $\frac{\sigma}{\delta} = 0.65$ (Fig. S9).

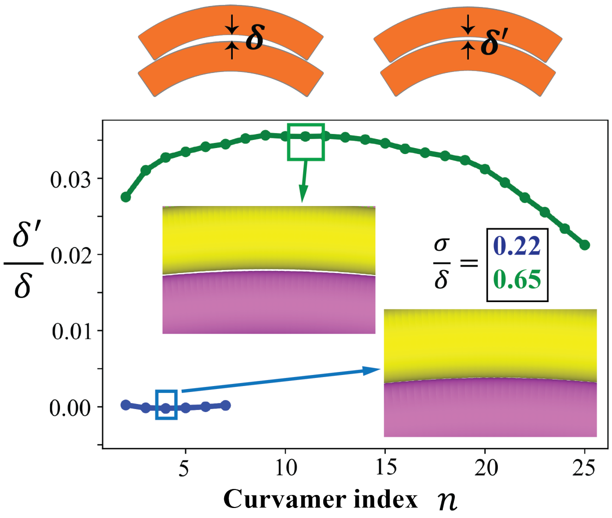


Figure S9: Gaps between $n$-th and $n+1$-th curvamer in the two stacks plotted as a function of curvamer position index. The magnified image of the gap between the 10th and 11th curvamer in the large stack ($\sigma/\delta = 0.65$) shows a small gap opening compared to the conformal contact between the 3rd and 4th curvamer in the small stack ($\sigma/\delta = 0.22$).

The escape through long-ranged interaction was investigated using the energy per curvamer plots as shown below in Fig. S10. The largest stacks found in these plots – $N_{min} = 69$ for $\sigma/\delta = 0.22$,

$N_{min} = 39$ for $\sigma/\delta = 0.43$, and $N_{min} = 25$ for $\sigma/\delta = 0.65$ correspond to the largest $H$ values shown on the plots of Fig. 4a in the main manuscript.

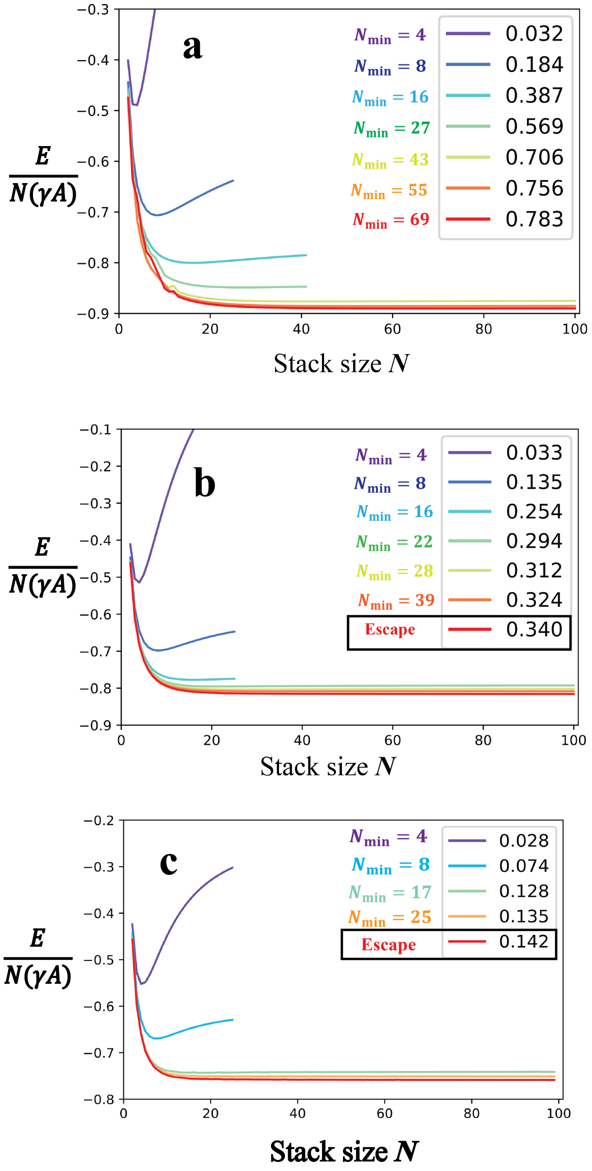


Figure S10: **(a)** Energy per curvamer plots as a function of stack size for different values of S ($\sigma/\delta = 0.22$). Because of the short-ranged interaction, stack size as large as $N_{min} = 69$ is observed for $S = 0.783$. **(b)** Energy per curvamer plots as a function of stack size for different values of S ($\sigma/\delta = 0.43$). No energy minimum was found while searching for stack size up to $N = 100$ for $S = 0.340$, resulting in an escape at a smaller value of $S$ compared to the case of (a). The largest possible stack size in this case is $N_{min} = 39$. **(c)** Energy per curvamer plots as a function of stack size for different values of S ($\sigma/\delta = 0.65$). The largest stack found in this case is even smaller ($N_{min} = 25$) at $S = 0.142$.
